# Supplementary material for: Solving estimating equations with copulas
Source: arXiv:1801.10576 source file (2022-08-19)
Supplement: Supplementary file 1 [file appendix.tex]

%!TEX root = ../copula_ee.tex

\section{Assumptions}
\label{sec:assumptions}
\begin{assumption}\label{asm:a1}
	The estimator $\what$ satisfies $\vert \what (\by) -  \wtrue (\by)\vert \to_P 0$ for all $\by \in \Ycal$.
\end{assumption}
\begin{assumption}\label{asm:a2}
	There is a class of weight functions $\Wcal$ and $\delta > 0$ such that
	\begin{subassumption}
		\item\label[assumption]{asm:a2i}  the class $\left\{ g_{\theta}w \colon  \| \theta - \thtrue \|_{T} < \delta, w \in \Wcal \right\}$ is $P$-Donsker,
		\item\label[assumption]{asm:a2ii} $\Prob(\what \in \Wcal) \to 1$.
	\end{subassumption}
\end{assumption}
\begin{assumption}\label{asm:a3}
	There exists $\thtrue \in \Theta$ such that $E\{\gtrue(\bY)\wtrue(\bY)\} = 0$ and, for any $\epsilon > 0$, \\ $\inf_{|\theta_t - \thtruet| > \epsilon, t\in T} \vert E\{g_{\theta, t}(\bY)\wtrue(\bY)\} \vert > 0$.
\end{assumption}
\begin{assumption}\label{asm:a4}
	The map $\theta \mapsto g_{\theta}$ is continuous in $L_2(P)$ at $\thtrue$.
\end{assumption}
\begin{assumption}\label{asm:a5}
	The map $\theta \mapsto \E\{g_{\theta}(\bY)\wtrue(\bY)\} $ is Hadamard differentiable in a neighborhood of $\thtrue$ and the derivatives $\Vtrue$ are invertible.
\end{assumption}
\begin{assumption}\label{asm:a6}
	There exists a sequence of continuous functions $w_{n}\colon \R^{2d + p} \to \R$ and $r_n^{-1} = O(1)$ such that
	\begin{align*}
		\sup_{\by} \biggl\vert \what(\by) - \frac{1}{n} \sum_{i=1}^n w_{n}(\by,\bY_i,\bX_i)  \biggr\vert = o_P\bigl(n^{-1/2}r_n\bigr).
	\end{align*}
\end{assumption}
\begin{assumption}\label{asm:a7}
	The class $\omegan = \left\{\omegant: t \in T \right\}$ where
	$\omegant(\by, \bx) = r_n^{-1} \E \bigl\{\gtruet(\bY) \wn(\bY, \by, \bx)\bigr\}$ for all $(\by, \bx) \in \Ycal \times \Xcal$ is $P$-Donsker\footnote{
		Since the function class changes with $n$,
		the definition of $P$-Donsker in this case is in the supplementary.}.
\end{assumption}
\begin{assumption}\label{asm:a8}
	The bootstrap estimator $\wboot$ satisfies $\vert \wboot(\by) - \wtrue(\by)\vert \to_P 0$ and $\Prob(\wboot \in \mathcal{W}) \to 1$ with $\mathcal{W}$ is as in \Cref{asm:a2}.
\end{assumption}

A discussion of the assumptions and sufficient conditions that may be easier to verify can be found in the supplementary materials.
